# Supplementary material for: Demographic Parity: Mitigating Biases in Real-World Data
Source: arXiv:2309.17347 source file (2023-09-27)

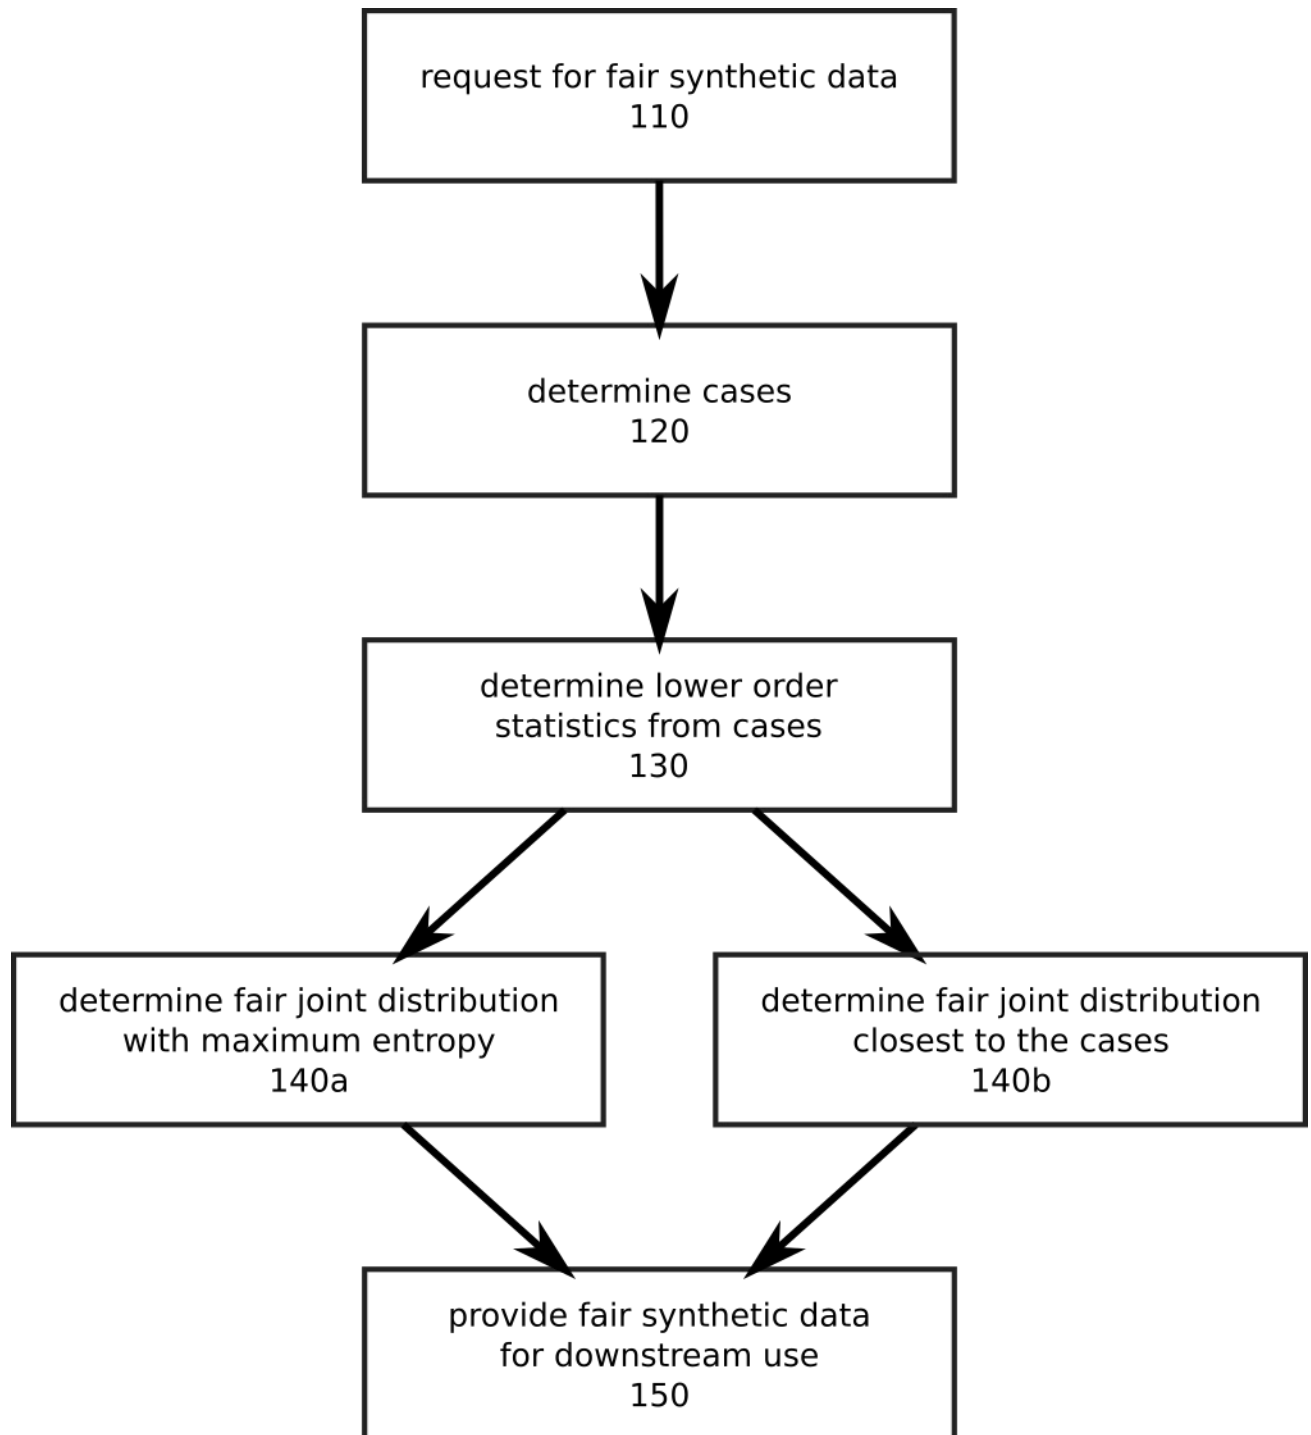

Figure 1: Synthetic data generation process.

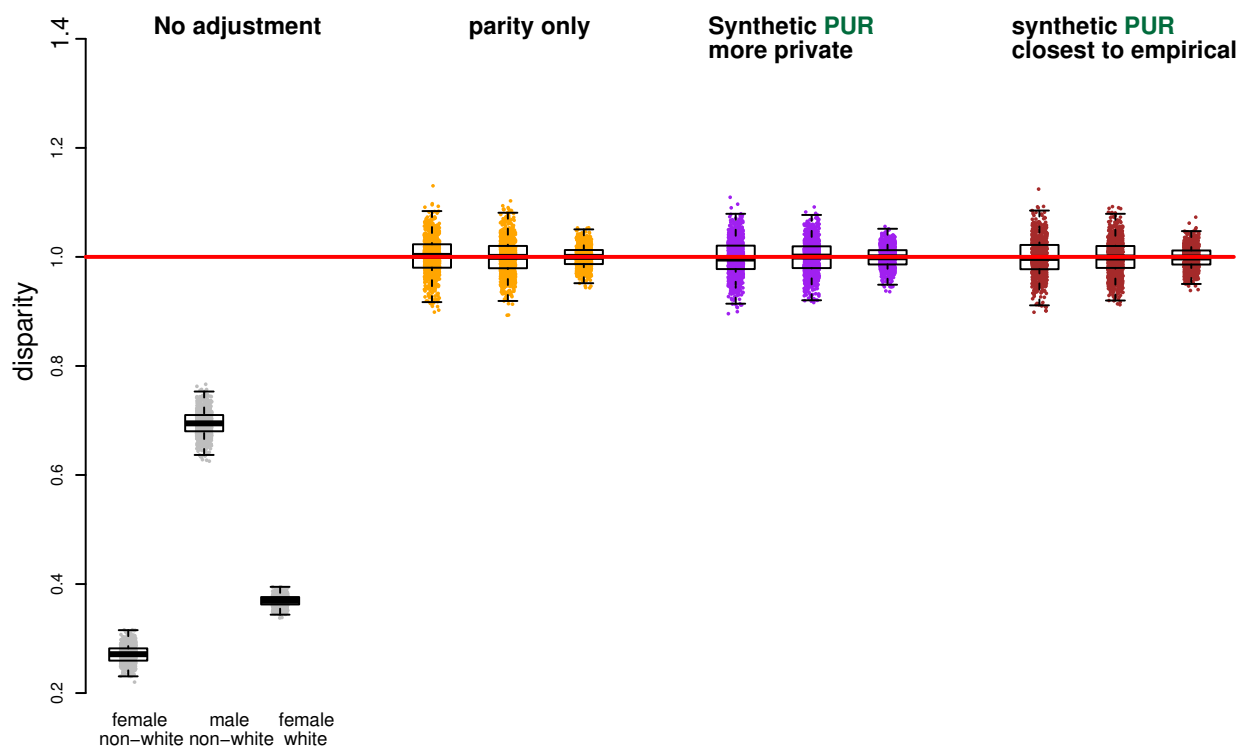

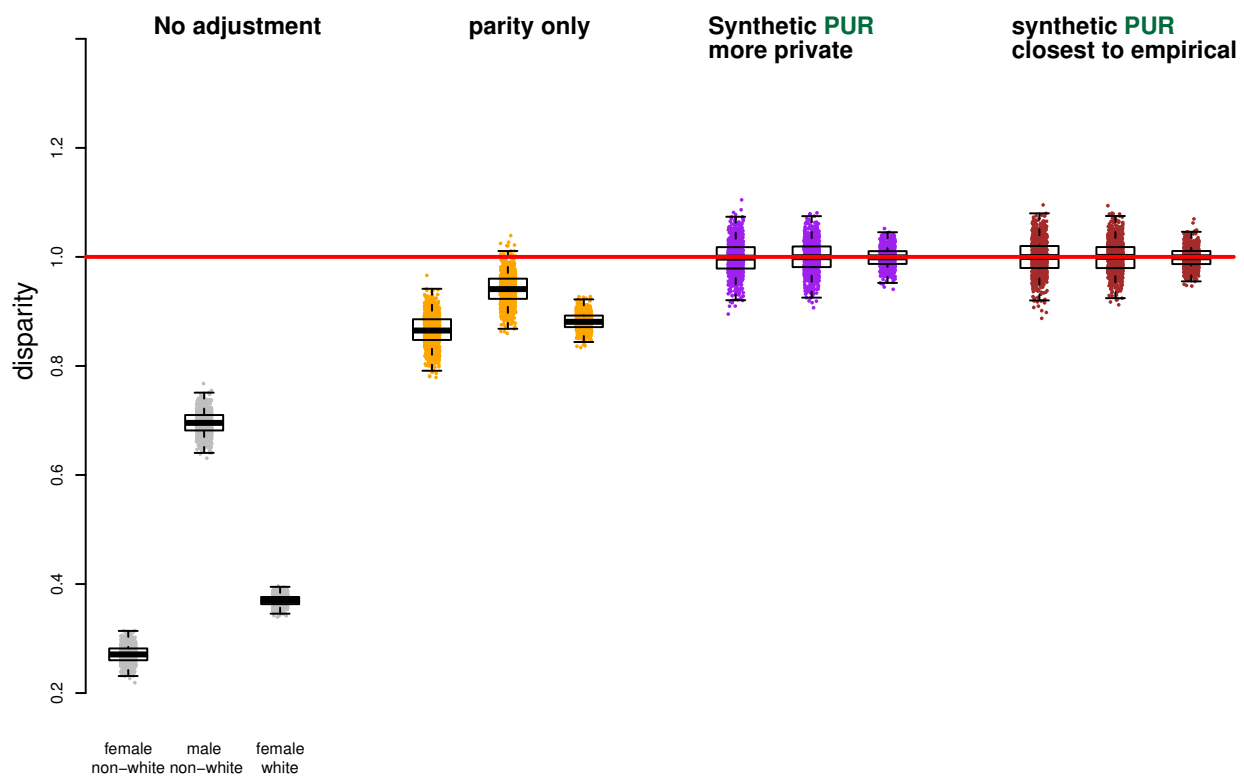

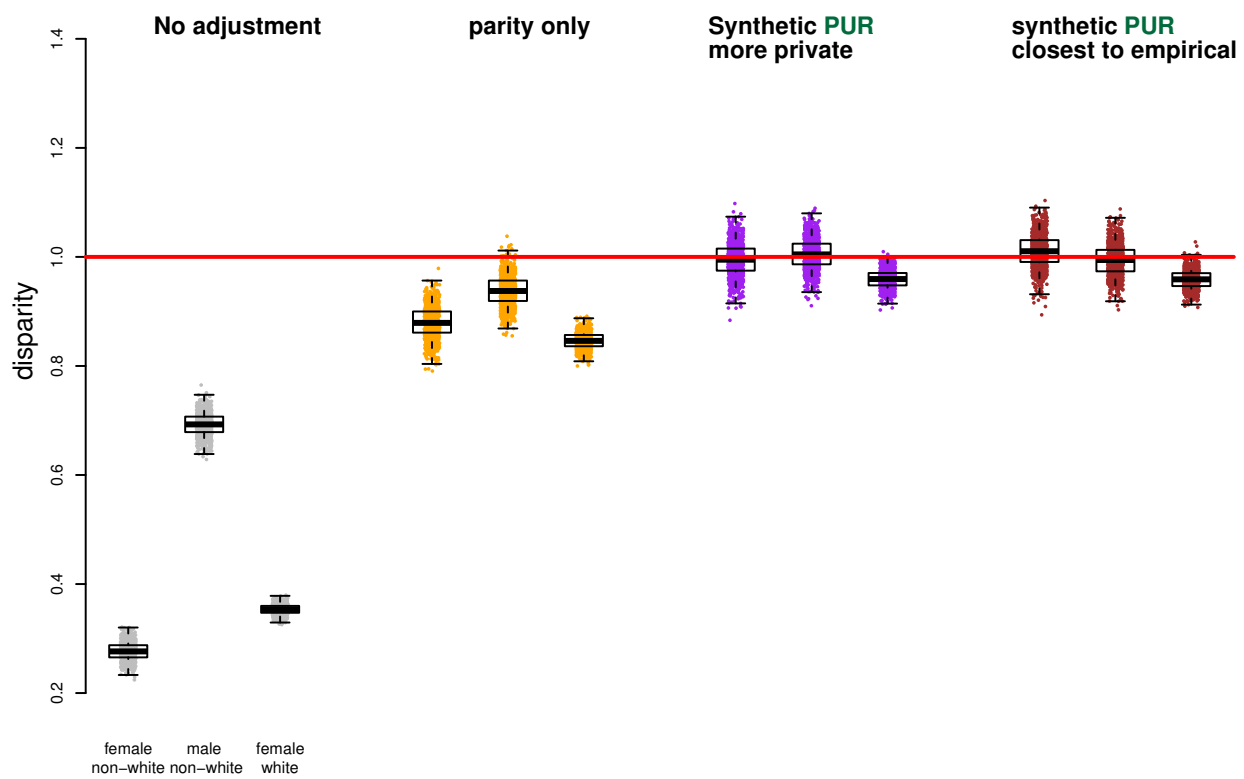

Supplement: Supplementary file 2 [file US_synthetic-data.pdf]
